# Supplementary material for: Vortex arrays and ciliary tangles underlie the feeding-swimming tradeoff in starfish larvae
Source: arXiv:1611.01173 ancillary file (2017-02-13)
Supplement: Supplementary file 1 [file starfish_paper_supps.pdf]

# Supplementary Materials for "Vortex arrays and ciliary tangles underlie the feeding–swimming tradeoff in starfish larvae"

William Gilpin[1], Vivek N. Prakash[2], Manu Prakash[2*]

[1]Department of Applied Physics, [2]Department of Bioengineering,

Stanford University, Stanford, CA

[*]To whom correspondence should be addressed; E-mail: manup@stanford.edu

February 12, 2017

# Contents

**1 Methods** **2**

A Culturing and imaging of starfish larvae . . . . . . . . . . . . . . . . . . . . . . 2

B Temperature control measurements . . . . . . . . . . . . . . . . . . . . . . . . 4

C Particle Image Velocimetry . . . . . . . . . . . . . . . . . . . . . . . . . . . . 6

D Principal Component Analysis . . . . . . . . . . . . . . . . . . . . . . . . . . 6

E Least Squares Fitting . . . . . . . . . . . . . . . . . . . . . . . . . . . . . . . 7

**2 Supplementary Tables and Figures** **9**

**3 Analytic and numerical models of feeding and swimming** **13**

A Validity of the Low Reynolds number approximation . . . . . . . . . . . . . 13

B Validity of two-dimensional polar swimmer . . . . . . . . . . . . . . . . . . . 14

C Solution of Stokes' Equation for a ciliated swimmer . . . . . . . . . . . . . . 15

C.1 Energetic properties of the squirmer model . . . . . . . . . . . . . . . 17

D Description of larval model: The "two mode" squirmer . . . . . . . . . . . . 18

E Description of geometric capture cross section . . . . . . . . . . . . . . . . . 20

E.1 Comparison with other feeding metrics . . . . . . . . . . . . . . . . . 24

F Description of particle capture simulation . . . . . . . . . . . . . . . . . . . . 26

F.1 The effects of random noise . . . . . . . . . . . . . . . . . . . . . . . 27

# 1 Methods

## A Culturing and imaging of starfish larvae

*Patiria miniata* embryos were spawned by injecting adult bat stars with 1-methyladenine, causing the release of gametes, which were then fertilized and allowed to develop over an 8 week period. Within a few days, the embryos first develop cilia and begin to rotate rapidly,

and within 4-5 days they enter the bipinnaria stage and begin swimming. Within several weeks they enter the brachiolaria stage, where they gradually develop a rudiment before entering a sessile juvenile form. The experiments focused on animals that were within the same developmental stage, synchronized to within a two-week period.

Culturing and feeding conditions matched standard practices in the field,,[1–4] as well as the conditions of the adult collection site in Monterey Bay, California. These parameters are shown in Table 1. Basic larval developmental parameters were also measured for several 8 week old starfish during the first day of experiments, and these parameters are given in Table 2

Animals were mounted in sea water on glass slides, with the circumoral field facing upwards, and then confined using a coverslip with clay protrusions to prevent the organism from being squashed. The height of the coverslip was slowly lowered until the animal was no longer able to swim (height of 450-550 $\mu$m depending on the larvae width). Animals were imaged using dark field microscopy on a Nikon TE2000-U microscope with an ORCA-Flash4.0 camera. For particle tracking experiments, images were recorded at 20 fps and 50 ms exposure, and for cilia imaging speeds of up to 800 fps were used.

The height of the chamber was sufficient that the flows near the midplane were unimpeded by wall effects, which was confirmed by three control experiments: (1) comparison of the flow fields across different z-planes (Figure S2), (2) analyzing the currents created by animals held stationary by a pipette (but away from walls), and (3) analyzing the flow fields generated by animals that were allowed to swim freely (Figure S1). For the latter, a video of a free swimming larva was taken in a Petri dish with a 10x Nikon inverted microscope. The filtered seawater in the dish was seeded with the same 1 : 100 dilution of 6 $\mu$m beads used in the confined experiment. Particle image velocimetry was performed on the resulting data, and the center-of-mass motion was subtracted out in order to generate a velocity field for the comoving frame of the animal. Simulated streamlines were then plotted and compared to the results for confined organisms (Figure S1).

In order to control for the effect of muscle contractions, a control experiment was performed with free-swimming larvae that spent an hour in a solution with a high concentration of magnesium ions (the salinity was matched with that of the original culture).[5] The magnesium ions are believe to inhibit nervous control of muscle actuations,[5, 6] leading the swimming larvae to repeatedly collide with each other and become locked together due to their inability to turn and reverse direction. Importantly, the forward swimming patterns remain the same, suggesting that the swimming is predominantly governed by ciliary actuation and not muscle activity.

## B Temperature control measurements

The larvae are cultured in a Darwin incubator (KB055-AA-LT) with an internal thermostat that reports a temperature of $14.9 \pm 0.5$°C. Separate measurements using a Fluke 62 Mini hand-held IR temperature probe find temperatures around the culture to be $14.8 \pm 1$°C (20 measurements) and additional measurements with a mercury thermometer record $15.3 \pm 1.1$°C (5 measurements).

The microscope room in which experiments are performed is temperature controlled. The internal thermostat measures $22 \pm 3$°C, with most variation throughout the day occurring due to airflow and foot traffic. Separate measurements using the handheld IR probe and mercury thermostat yielded temperatures of $22.5 \pm 0.5$°C (15 measurements) and $22.8 \pm 1.0$°C (5 measurements). These measurements were performed in the typical location of a slide or Petri dish on the microscope stage with the light source turned "on."

Upon exiting the incubator and being placed in the experimental apparatus, the larvae are expected to slowly warm from their initial temperature ($\sim$ 15°C) until they asymptotically reach the temperature of the microscope room ($\sim$ 22°C). In order to test this hypothesis, a mock experiment was performed in which time-resolved water temperature measurements were periodically taken with a Omega CDH45 hand-held temperature and salinity probe. The resulting sequence of measurements is shown in Figure S3, and the

reference measurements for the incubator and microscope room are overlaid on the plot.

The measurements may be fit to Newton's law of cooling,

$$T(t) = T_{room} - (T_{room} - T_{incubator}) \exp(-rt) \tag{A1}$$

where $r$ is a constant inversely proportional to the effective heat capacity of the entire experimental setup. The best fit is underlaid in Figure S3. For the experimental setup, $r = .077\ s^-1$, $T_{room} = 22.12$°C and $T_{incubator} = 15.86$°C. These asymptotes are also shown in the Figure.

We note that the first data point taken by the water probe, and subsequently the lower asymptote of the best fit to Newton's law of cooling, are greater than the starting values measured in the incubator. This is likely because the first measurement is taken only after 5 mL of water has been pipetted out of the incubated culture and into a small cuvette (a cuvette is used instead of a slide in order to ensure that the prongs of the temperature meter can be fully submerged). We thus attribute this effect to collective heating of the small water volume due to transfers between containers and mixing due to the pipette. Subsequent measurements show a uniform, asymptotic increase in temperature as the sample gradually warms to room temperature, a process that takes about 90 minutes.

All experiments reported in the manuscript occur over intervals shorter than the first five minutes after the larvae exit the bulk culture (indicated by an inset in the Figure). During this time, the slide warms at an initial rate of $\approx 0.4$°C$/min$, or about 2°C for a typical experiment. This means that both the absolute change in temperature is small during our experiments, and that the larva does not incubate at the different temperature long enough for physiological changes to manifest. Other studies of the effect of temperature variation on larval behavior suggest that invertebrate larval swimming only noticeably reacts to temperature changes of around 10°C, suggesting that experiments with the short timescale reported here are not affected by the temperature variation on the microscope stage.[7, 8] We

also note that both the upper and lower temperatures, 15°C and 23°C, are well within acceptable bounds for echinoderm larval cultures.

## C Particle Image Velocimetry

Particle Image Velocimetry (PIV) fields were generated using OpenPIV for Python.[9] Field parameters were optimized based on the 1 : 100 bead dilution used in the flow field visualization experiment experiments, and then held constant across all analyses in order to reduce systematic errors due to inconsistent discretization. For experiments where time variation was not observable in the resulting vector fields, velocity fields were averaged across time using a running median filter to remove outliers. PIV parameters are given in Table 3.

## D Principal Component Analysis

In order to extract quantitative measurements of behavior, Principal Component Analysis (PCA) was applied to data sets consisting of time series of two-dimensional vector fields generated by PIV. For a movie with $N$ frames and a PIV field defined at $M \times M$ points in the image, a covariance matrix was generated by taking the inner product of $M^2$ vectors with length $2N$ corresponding to the two components of the velocity field at each point.The eigenvectors of this matrix are ranked by the magnitude of their associated eigenvalues, and the first K eigenvectors are the K principal components. This process was performed using the Python package scikit-learn.[10] The amplitude of each principal component versus time was then calculated by taking the sum of the inner product of the PIV field at each timepoint with each of the principal components.

The first two principal components are shown in Figure S4. The two components are anti-correlated. We interpret the first mode as the "swimming mode" due to its high agreement with the time-dynamics of the first-order squirmer mode (discussed in the main text). The second mode has lower overall speeds associated with it, and it contains six characteristic features spaced across the animal's perimeter that match the locations of the vortices visible

during the feeding period of the time series: two pairs of vortices at the front and back of the animal, and two smaller features near the animal's midsection.

We note that the PCA modes result from unsupervised extraction of anti-correlated components from the finite time series. Thus while each of the two PCA modes may individually comprise a superposition of infinite squirmer modes, the two PCA modes nonetheless remain orthogonal due to the requirements of the PCA algorithm. In particular, the "swimming" mode appears to have prominent fore/aft asymmetry characteristic of a non-zero $B_2$ or "pusher/puller" component being present in addition to the $B_1$ component that generates thrust.

# E Least Squares Fitting

Least squares fitting to the admixture of basis functions in the squirmer model (described in the next section) was performed using the Mathematica function LinearModelFit[]. Because the squirmer model allows an infinite number of terms in the set of coefficients $\{B_i\}$, the number of allowed terms in the series was truncated. This matches the empirical observation that the average amplitude of higher order terms generally decreases rapidly with increasing $i$, which results from the physical constraint that a realistic squirmer cannot access arbitrarily high-order terms in the squirmer model due to physical limitations in the level of spatial resolution it can impose when creating velocity boundary conditions on its surface. Fitting was done separately for the x and y components of the velocity field generated by PIV, and the two fits were checked for concordance. Fitting was performed for 10, 20, and 50 terms, and all cases yielded similar relative amplitudes for the first ten modes.

In any movies for which drift or rotation of the swimmer's body was observed to occur, rigid body registration parameters were extracted using the Fiji Plugin Virtual Stack Registration (with the rigid setting enabled). At each timepoint, these parameters were used to appropriately translate and rotate the analytic basis functions before fitting them to the PIV field for that timepoint.

For the PIV time series for a starfish larva shown in Figure 4 of the main text, simulations were performed in order to calculate the instantaneous particle capture cross section for the "best fit" squirmer model at each timepoint (the simulations and cross section are defined below). This allowed calculation of the time-resolved capture cross section for the larva shown in the time series (Fig. S5). Comparing this value to the swimming speed (which is proportional to the first-order mode in the squirmer model), it is apparent that the geometric capture cross section increases when the animal reduces its speed.

# 2 Supplementary Tables and Figures

**Table 1** Larva culturing conditions.

| Parameter | Value |
|---|---|
| Water temperature | 15°C |
| Water salinity | $3.0 \pm 0.2\%$ |
| Culture animal density | $< 0.1$ larva/mL |
| Water cleaning rate | 2 per week |
| *Rhodomonas lens* culture density | 5 million cells/mL |
| *Dunaliella tertiolecta* culture density | 1.5 million cells/mL |
| Algae Feeding frequency | 10 mL/strain per 1 L culture every 2 days |
| Larva age during experiments | 8-9.5 weeks |

Algae densities measured using a calibrated Secchi disk.

**Table 2** Morphometrics for 22 individuals measured on a single day, 8 weeks after spawning.

| Parameter | Value |
|---|---|
| Long axis length | $1200 \pm 200\ \mu m$ |
| Middle width (tip to tip) | $800 \pm 100\ \mu m$ |
| Side lobe protrusion | $130 \pm 40\ \mu m$ |
| Aspect ratio | $1.56 \pm 0.11$ |
| Arm length/body width | $0.11 \pm 0.02$ |

Measurements and calibration performed using ImageJ.

**Table 3** Parameters used in PIV analysis.

| Value | Parameter |
|---|---|
| Extension window | 100 px |
| Overlap window | 30 px |
| Interrogation window | 60 px |
| Temporal averaging | 60 frames (3 s) |
| Time step | 0.05 s |

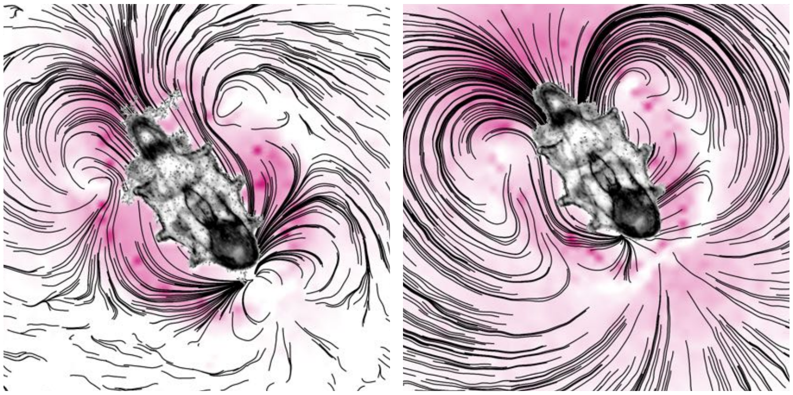

**Figure S1 Flow fields of a free-swimming larvae.** Computed streamlines from PIV data of a freely-swimming animal at two different timepoints, with the magnitude of the velocity field underlaid.

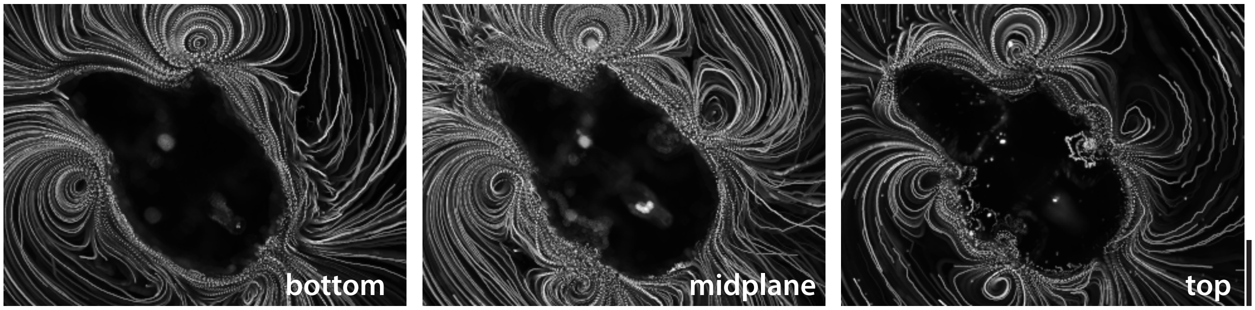


**Figure S2 Minimal z-variation of the vortex structure.** For an organism confined in a chamber and imaged with fluorescent beads, vortices persist across three different z-positions along the chamber height (60 s projections of a 12 fps video, Scale bar 50 $\mu$m).

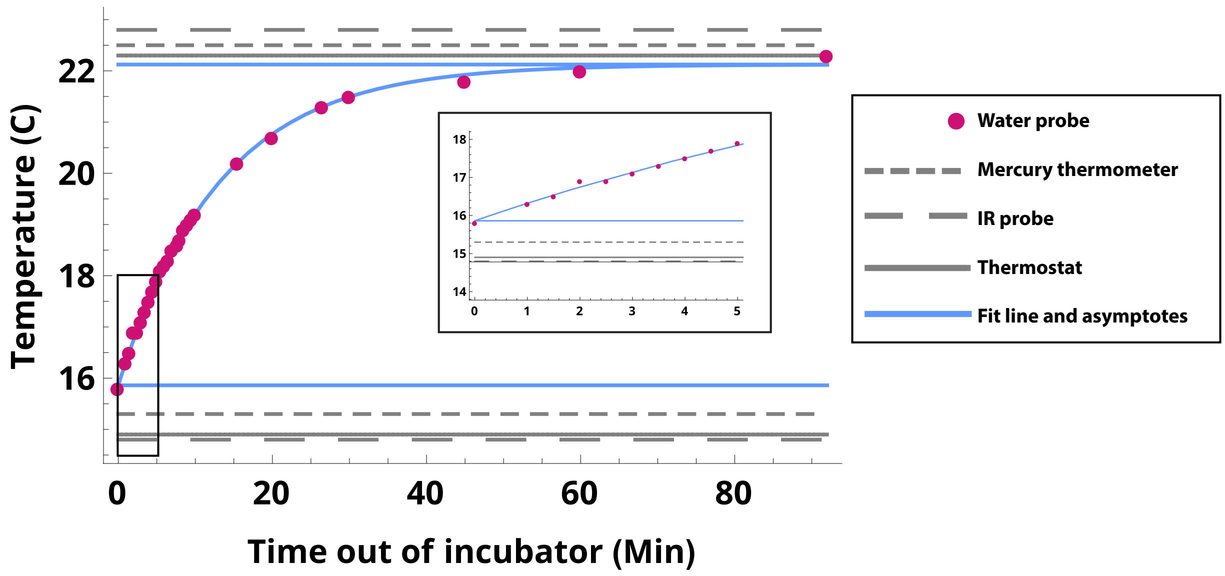


**Figure S3 The temperature of the larval environment after removal from incubator** Separate measurements of the incubator and the microscope area were taken with thermostats, an IR monitor, and a mercury thermometer (as indicated in the legend). Time-resolved measurements were taken with handheld water probe. A best fit to Newton's law of cooling is underlaid as a solid line. Inset shows the first five minutes (a typical experiment timescale).

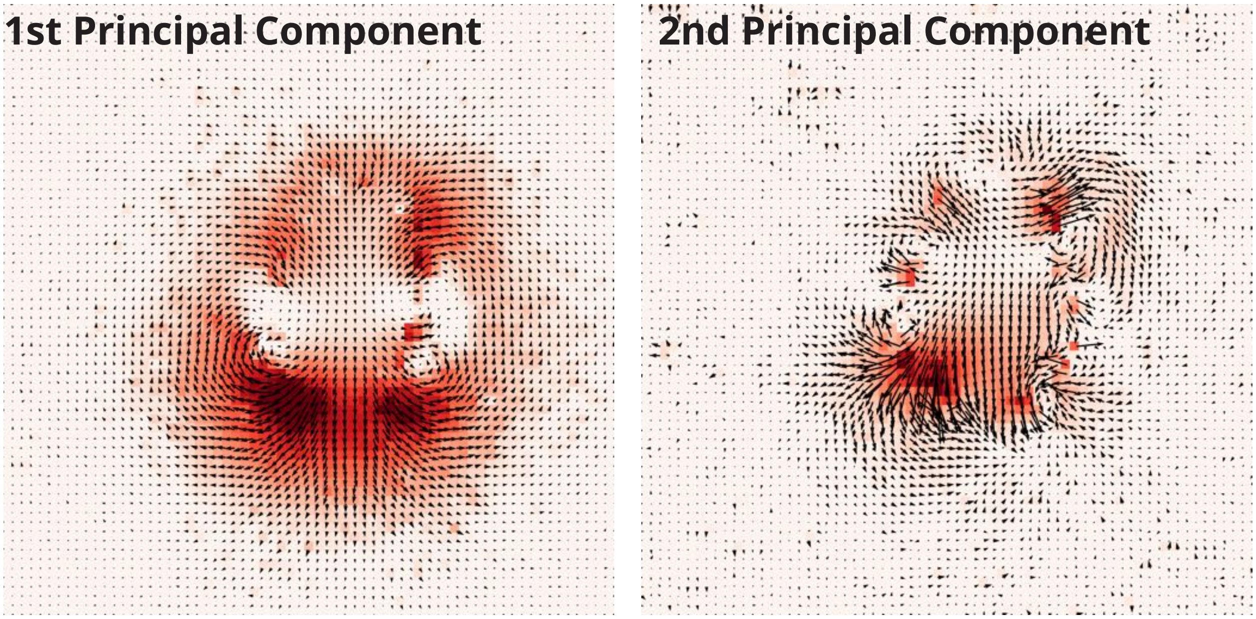


**Figure S4 The first two principal components of a time-varying larval flow field.** The first two principal components of the PIV time series shown in Figure 4. The vector field is shown in black, and the velocity magnitude is underlaid in color.

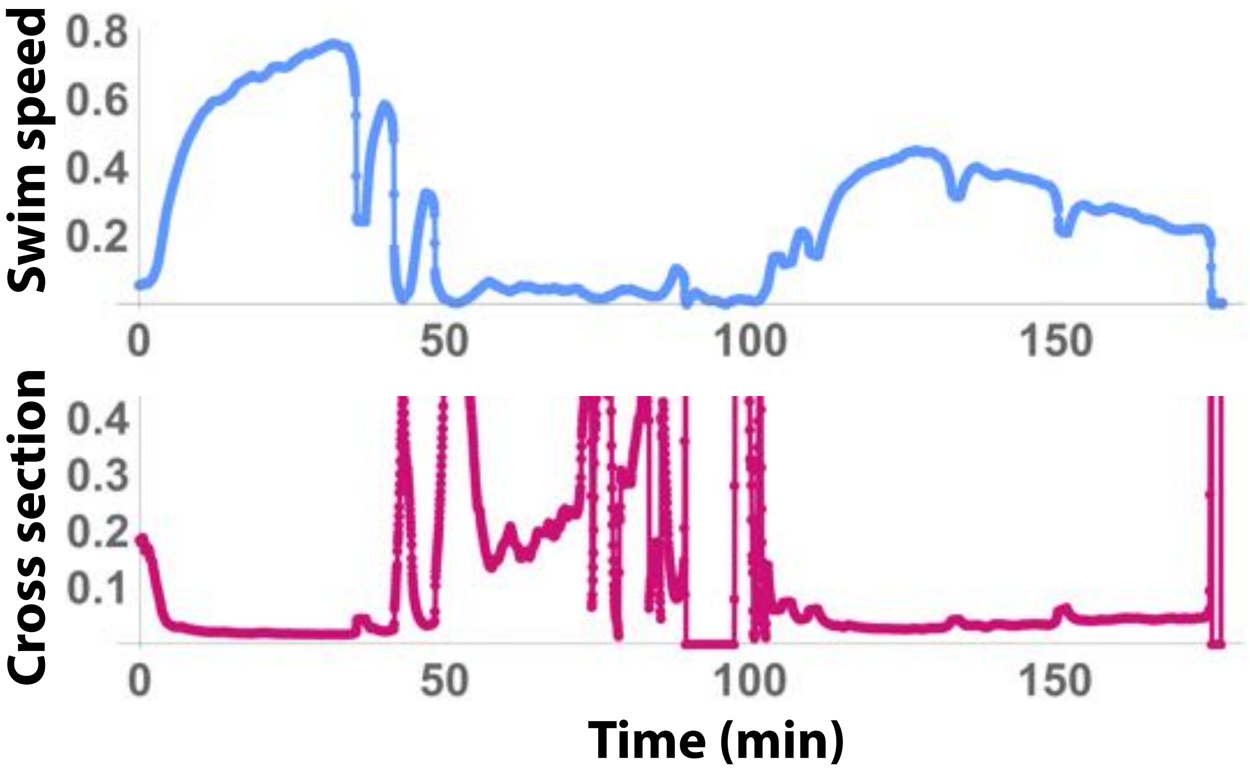


**Figure S5 The time-resolved capture cross section of a starfish larva.** For the best-fit squirmer model for each timepoint of the movie shown in Figure 4, a particle capture simulation was performed in order to calculate the instantaneous particle capture cross section. The best-fit first-order mode is shown in the top panel (representing the swimming speed), and the cross section is shown in the bottom panel. The vertical axis units are arbitrary, and they do not affect the inverse correlation between the two measurements.

# 3 Analytic and numerical models of feeding and swimming

## A Validity of the Low Reynolds number approximation

The aspect ratio of a typical starfish larvae is compact; rarely does one dimension exceed the length of the others by more than a factor of 2. In order to determine the validity of the Stokes' flow approximation, we first treat the larvae as a sphere in a viscous flow, using for the radius, $a$, of the sphere the **maximum** observed dimension of the organism (so as to overestimate the Reynolds number).

$$Re = \frac{v_{max} a}{\nu}$$

where $\nu$ is the kinematic viscosity of seawater, $\nu \approx 1.0 \times 10^{-6}$ m$^2$ s$^{-1}$, $v_{max}$ is the maximum speed of the swimmer, and $a$ is the characteristic length scale of the problem. The maximum bat star larvae length observed in the experiments corresponds to $a = 1.0$ mm; the maximum observed swimming speed was 1/2 of a body length per second, $v_{max} = 0.5$ mm/s for the largest specimen. This corresponds to a maximum Reynolds number for a free swimming starfish larva

$$Re = \frac{500 \times 10^{-6}\ 10^{-3}}{10^{-6}} = 0.5$$

Because all quantities were estimated conservatively from their maximum values observed at any point during the experiments, this calculation provides an upper bound on the Reynolds number for our experimental system. Real values observed at any given time during the experiments were a tenth of this estimate or lower. For the 6 $\mu$m beads and $\sim 5.5$ $\mu$m algae advected by the larvae's flow field, the characteristic length scale $a$ is much smaller,

$$Re = \frac{500 \times 10^{-6}\ 6 \times 10^{-6}}{10^{-6}} = 0.003$$

For the experiments described in the text, the swimming larvae is immobilized, making the latter quantity the true Reynolds number for the experimental system. However, because a large, maximally swimming larvae can achieve Reynolds numbers of $0.5 \sim 1$, a boundary layer may occur near the organism of size $\sim a/Re$, outside of which inertial effects become important. However, the high order vortices observed in the experiments were confined to within one body length, and so intermediate Reynolds number swimming could only affect the far field swimming/recirculation term observed in confined organisms.

For the ultra near-field, another Reynolds number may be described corresponding to that of the beating cilia[11]

$$Re = \frac{\omega L r_0}{\nu}$$

where $\omega$ is the beat frequency, $L$ is the length, and $r_0$ is the width. Using the largest $L$ and $\omega$ separately observed for any measured cilium, $L \approx 40\mu$m and $\omega \approx 7$ Hz, and a conservatively-estimated width of $r_0 = 1\ \mu$m,

$$Re \approx 0.0003$$

Because all quantities were estimated conservatively from their maximum values observed at any point during the experiments, this calculation again provides an upper bound on the Reynolds number for our experimental system.

## B Validity of two-dimensional polar swimmer

Because of the large z-height of our imaging device compared to typical water-based microfluidic cells, the flow was modelled as a 2D Stokes' flow. This was further verified by changing the focal plane of the imaging and finding that the flow field stays the same, establishing that gradients in velocity components along the xy-plane were greater than those along the z axis (wall effects are further discussed in the supplementary experiments section).

We thus model swimming using a cylindrical, rather than spherical squirmer model. This

distinction is particularly important because our animal has bilateral symmetry across an axis normal to the imaging axis, as well as strong localization of currents within the area of the ciliary band, which is not uniform across the azimuthal coordinate. We note that the flow field induced by a cylindrical squirmer is qualitatively similar to the one described by Pepper et al. (2012) for a confined squirmer when even stronger wall effects (in the form of a true Hele-Shaw geometry) are present. However, because the height of our device is the body width, and the near-field effects we observe are confined to within only a few body widths, we do not expect Hele-Shaw wall effects to dominate the feeding currents.

## C Solution of Stokes' Equation for a ciliated swimmer

At low Reynolds number in two dimensions, Stokes' equation reduces to the biharmonic equation,

$$\nabla^4 \psi = 0 \tag{A2}$$

where $\psi$ is the streamfunction for the organism, commonly defined as the vector potential for the velocity field,

$$\nabla \times (\psi \hat{\mathbf{z}}) = \mathbf{v} \tag{A3}$$

Using polar coordinates, this equation becomes

$$v_r = \frac{1}{r}\frac{\partial \psi}{\partial \theta}$$
$$v_\theta = -\frac{\partial \psi}{\partial r}$$

The general solution of (A2) is the Michell series,

$$\begin{aligned}\psi(r,\theta) &= a_0 r^2 + b_0 r^2 \ln(r) + c_0 \ln(r) + d_0\theta \\ &+ \Big(a_1 r + b_1 r^{-1} + b_1^{'} r\theta + c_1 r^3 + d_1 r\ln(r)\Big)\cos\theta \\ &+ \Big(e_1 r + f_1 r^{-1} + f_1^{'} r\theta + g_1 r^3 + h_1 r\ln(r)\Big)\sin\theta \\ &+ \sum_{n=2}^{\infty}\left(a_n r^n + b_n r^{-n} + c_n r^{n+2} + d_n r^{-n+2}\right)\cos(n\theta) \\ &+ \sum_{n=2}^{\infty}\left(e_n r^n + f_n r^{-n} + g_n r^{n+2} + h_n r^{-n+2}\right)\sin(n\theta) \qquad \text{(A4)}\end{aligned}$$

Using (A3) and dropping all terms that diverge as $\mathcal{O}(r)$ or faster as $r \to \infty$ (because the area element scales as $r$),

$$\begin{aligned} v_r(r,\theta) &= \frac{1}{2}B_1\cos\theta\left(\left(\frac{a}{r}\right)^2 + \log(r/a) - 1\right) + \sum_{n=2}^{\infty}\frac{n}{2}B_n\cos(n\theta)\left(\left(\frac{a}{r}\right)^{n+1} - \left(\frac{a}{r}\right)^{n-1}\right) \\ v_\theta(r,\theta) &= \frac{1}{2}B_1\sin\theta\left(\left(\frac{a}{r}\right)^2 - \log(r/a)\right) + \sum_{n=2}^{\infty}\frac{1}{2}B_n\sin(n\theta)\left(n\left(\frac{a}{r}\right)^{n+1} - (n-2)\left(\frac{a}{r}\right)^{n-1}\right) \end{aligned} \qquad \text{(A5)}$$

where coefficients of similar terms have been grouped into a new set of coefficients. We note our solution is equivalent to Blake's classic solution for a squirmer in cylindrical coordinates, with an additional set of terms $\pm(1/2)B_1\log(r/a)$ that diverge logarithmically in the far-field $r \to \infty$, which account for the immobilization of the squirmer and the recirculation it induces.[12] Unlike in Blake's original model, the immobilized swimmer has no drag force acting in a direction opposite its swimming velocity, and so a two-dimensional Stokeslet must be subtracted from Blake's solution—which both removes Blake's far-field constant velocity term and introduces the logarithmic factor. The latter term is a consequence of Stokes' paradox, and practically it means that these solutions are valid only for $r/a < \mathcal{O}(Re^{-1})$ ($r_{max} \gtrsim 30$ cm).[13] Recently, more advanced models have developed for the specific case of a squirmer in a Hele-Shaw geometry,[14] which show qualitatively similar results (the formation

of a large recirculation dipole). However, our imaging setup had coverslip heights of $450-550$ $\mu$m, well outside of the Hele-Shaw regime for the $\sim 400$ $\mu$m region around the body on which we focus, and so recirculation was more attributable to immobilization than wall effects. This was further verified by measuring the flow field in different z-planes to confirm that the top and bottom slides were not attenuating the flow near the mid-plane, as well as by analyzing the flow fields of unconfined, free-swimming animals.

For the simulations used to test feeding efficiency, a tethering term was not necessary, and Blake's exact original solution was used,[12]

$$v_r(r,\theta) = \frac{1}{2}B_1 \cos\theta \left( \left(\frac{a}{r}\right)^2 - 1 \right) + \sum_{n=2}^{\infty} \frac{n}{2} B_n \cos(n\theta) \left( \left(\frac{a}{r}\right)^{n+1} - \left(\frac{a}{r}\right)^{n-1} \right)$$
$$v_\theta(r,\theta) = \frac{1}{2}B_1 \sin\theta \left( \left(\frac{a}{r}\right)^2 + 1 \right) + \sum_{n=2}^{\infty} \frac{1}{2} B_n \sin(n\theta) \left( n\left(\frac{a}{r}\right)^{n+1} - (n-2)\left(\frac{a}{r}\right)^{n-1} \right) \quad \text{(A6)}$$

### C.1 Energetic properties of the squirmer model

Blake's original paper includes a calculation of the "rate of working" per unit area for the squirmer model,[12] which provides a measurement of the power investment required to sustain each mode in (A6),

$$R = \frac{\mu}{a}\sum_{n=1}^{\infty} R_n \qquad R_n = nB_n^2$$

where $a$ is the body width and $\mu$ is the viscosity. A plot of the value of each these terms $R_n$ with $B_n = \mu/a = 1$ is shown in Figure S6. We note that because the swimming speed scales with the first-order mode amplitude, $v_{swim} = (1/2)B_1$, the first-order term in this series matches the prediction of the Stokes' drag, $P_{drag} = F_{drag}v_{swim} \propto B_1^2$.

An alternative energetic calculation that takes into account the dissipation integrated over all space is the net power dissipation,[15] or enstrophy, which gives the dissipation due to the vorticity

$$P_{diss} = \mu \int_1^{\infty} \int_0^{2\pi} \omega(r,\theta)^2 r dr d\theta$$

Substituting the original cylindrical squirmer model (without the logarithmic term for con-

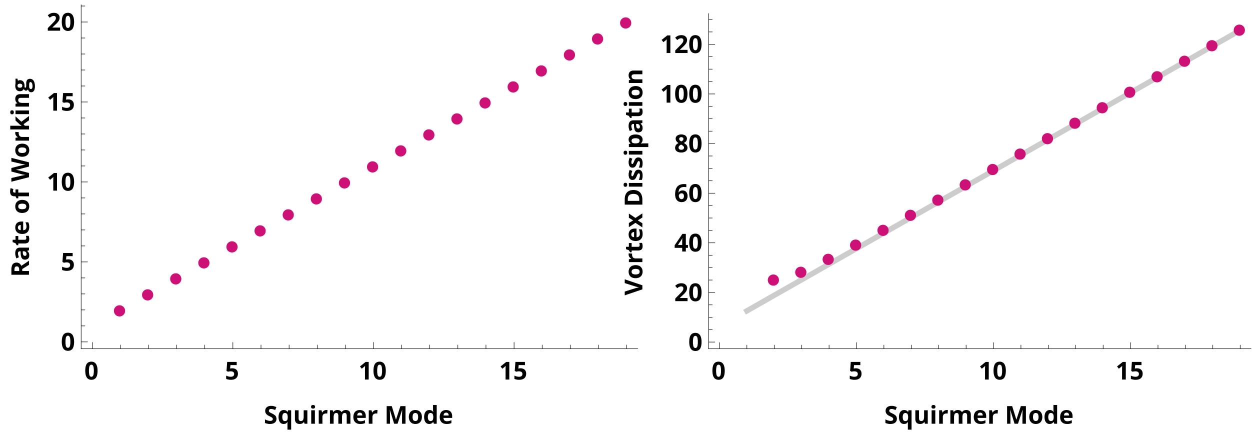


**Figure S6 The rate of working per unit area and vortex dissipation for the squirmer model.** Two measurements of the energetic cost of different modes in the squirmer model. For each mode, $B_n = 1$.

finement effects) results in an integral of a summation that can be rearranged as a summation of integrals. This allows a power dissipation for each term in the squirmer model to be defined, $P_{diss} = \sum_{n=2}^{\infty} P_{diss}^{n}$. Figure S6 displays first 20 terms in this series when $\mu = 1$ and $B_n = 1$ individually for each term, which provides the dissipation associated with drag in the vortex core for each term in the squirmer model. For large $n$, $P_{diss}^{n} \approx \mu 2\pi n$, underlaid on the plot.

Both energetic calculations included here suggest that the energetic cost to maintain modes of the same amplitude increases linearly with $n$.

## D Description of larval model: The "two mode" squirmer

For simulations, a model squirmer in the comoving frame was studied that did not include the immobilization terms in (A5). This squirmer corresponds to Blake's original free-swimming solution, (A6).

A set of "two-mode" model swimmers was constructed by setting all terms in (A6) equal to zero except for $B_1$ and $B_n$, where $n = 2, 3, 4, \ldots$. These squirmers represent minimal models of swimmers that generate fixed numbers of vortices using localized reversals of ciliary beat direction, with the number of vortices equaling $2n$ for $n$ sufficiently large (for

the constraints imposed below, $n \geq 5$, for $n < 5$, $N_{vort} = 2(n-1)$). These models thus have two free parameters, $B_1$ and $B_n$, which set the swimming speed and the size of the recirculation regions, respectively. The swimming direction is set without loss of generality by imposing $B_1 > 0$; however, $B_n$ can be either positive or negative. In order to facilitate direct comparison of model swimmers with different $n$, two constraints were be imposed:

*1.* **The maximum surface velocity must be the same for all two-mode swimmers.** Because the microscopic origin of the fluid flow is the same for all model squirmers, the maximum ciliary speed achieved anywhere on the squirmer's body must be the same. From (A6),

$$s_n^{max} \equiv \max(|v_\theta(r=a,\theta)| : \theta \in [0, 2\pi])$$

where $a$ is the squirmer radius. This results in a rescaling condition,

$$(B_1, B_n) \to (B_1/s_n^{max}, B_n/s_n^{max})$$

*2.* **The vorticity region must be the same size for all two-mode swimmers.** The "crossover" length scale that determines the size of the recirculation regions around the swimmer is determined analytically by finding the distance to stagnation points in the fore ($\theta = 0$) or aft ($\theta = \pi$) of the model swimmer. Setting (A6) equal to zero results in an equation for the stagnation points, which alternate appearing in front of and behind the swimmer,

$$r_n^s = \left(\frac{B_n}{B_1} n\right)^{1/(n-1)}$$

For the comparative simulations, this length scale is clamped $r_n^s = r_s$ for all $n$, resulting in a constraint equation

$$B_n = B_1 \frac{r_s^{n-1}}{n}$$

We note that this constraint is not a biological limitation, like constraint (1). Rather, because our figure of merit for evaluating larval feeding is a capture cross section, this geometrical

constraint must be imposed to ensure that different models encounter comparable total cross sections of the water column while swimming. Different $n$ models that scan the same total cross section of water will catch different fractions of particles present in the water column, leading to differences in their effective capture cross section.

Conditions (1) and (2) determine an infinite set of two-mode squirmers of various orders $n$ with swimming speeds given by $(1/2)B_1$. The feeding efficiency of these squirmers can then be calculated using a numerical simulation.

## E Description of geometric capture cross section

For a simulation of a line source of $N$ particles incident on a 2D swimmer, the two dimensional capture cross section is

$$\sigma = \frac{\sum_i^N p_i^{capture}}{\lambda}$$

where $\lambda$ is the line density of particles (in particles/meter) and $p_i^{capture}$ equals the total probability of a particle being captured during the simulation, which is run sufficiently long that all particles either are captured or move well past the body into the far field.

A requirement of "interception feeding" is that particles must pass very close to the surface in order to be successfully captured via a local ciliary reverse beat. We encode this requirement into the form of $p_i^{capture}$ by defining an annular capture region around the squirmer surface with a size given by $\delta$, the "interception distance"

$$p_i^{capture} = Q_i\Big(1 - \exp(-f\tau_i)\Big) \tag{A7}$$

where the arguments of $Q_i = Q_i(\delta/a, y_0/a)$ and $\tau_i = \tau_i(\delta/a, y_0/a)$ have been suppressed. $y_0$ is the initial coordinate of the simulated particle along the line source, which can be non-dimensionalized by the squirmer body width $a$. The quantity $Q_i$ is a binary membership function that equals one if particle $i$ passes within $\delta$ of the surface, and which equals zero if it does not. $\tau_i$ is the residence time, or the amount of time that a particle traveling along a

streamline will spend within $\delta$ of the surface when $Q_i = 1$. $f$ is a constant capture rate per unit time. The exponential term arises from solving the first-passage time problem of finding the probability of a particle being captured at any time during the interval $\tau_i$ that it travels within $\delta$ of the surface. In general, $Q_i$ and $\tau_i$ cannot be computed analytically from the squirmer model, and so we use high-resolution numerical simulations using the variable-step integrator described in the next section.

For interception feeders, the probability $f$ of a given particle being captured per unit time is very small, and so the exponential function in (A7) can be approximated as $\exp(-f\tau_i) \approx 1 - f\tau_i$. In this case, the capture cross-section for an interception feeder becomes,

$$\sigma = \frac{f\ \sum_i^N Q_i \tau_i}{\lambda} \tag{A8}$$

Where the arguments of the indexed quantities have again been suppressed. This quantity has units of length, as would be expected for a capture cross-section in a two-dimensional system.

(A8) is a complete expression for the two-dimensional cross section for the simulations presented in our paper. However, this quantity depends on the geometry of the simulation, leading it to increase when the simulation parameter $\delta$ increases. For small enough $\delta/a$, numerical work (Figure S7) confirms that the number of particles that pass within the interception distance increases linearly with $\delta$. This is an expected result, since intuition suggests that at small $\delta/a$, the capture cross section should be a smooth monotonic function in $\delta$, resulting in a leading-order linear term in a series expansion in $\delta/a$. Additionally, the summation in (A8) leads the total cross section to also scale linearly with $N$, the total number of particles used in the simulations. We take advantage of this linearity to divide out both $N$ and the linear dependence $(1 + \delta/a)$, in order to produce a "reduced" cross section

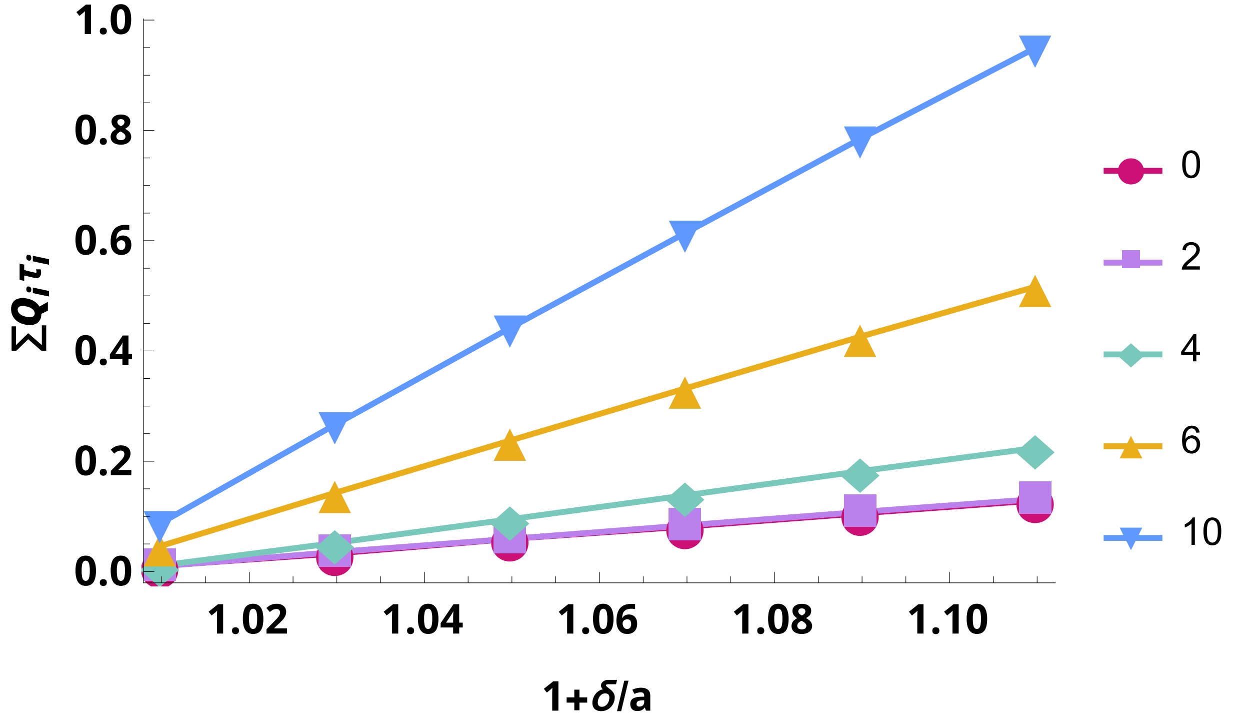


**Figure S7 The effect of varying the interception distance on the capture cross section.** The effect of changing the size of $\delta$ on the cross section defined in (A8), when the prefactors $\lambda$ and $f$ are set equal to one (units are thus arbitrary). The distinct colors/markers refer to the number of vortices generated by the five swimmers.

metric that does not depend on these simulation parameters,

$$\sigma^* = \frac{\sum_i^N Q_i \tau_i}{N} \frac{a}{a+\delta} \tag{A9}$$

where $N \propto \lambda$ is the initial number of particles used in the line source in the simulation, which is taken to be large enough that the results of the simulation do not vary as it is further increased (typically for a simulation box of size $L = 8a$, $N = 400$ particles, resulting in $\lambda = 50/a$). The remaining constants in (A8) are all set equal to one because they do not affect the relative performance of different squirmer models. The simplified version of the cross-section, $\sigma^*$, depends only on the geometry of the flow and is thus used as a measure of feeding ability for the two-mode squirmer model described above.

As noted in the main text, the increasing number of vortices resulting from successive "two

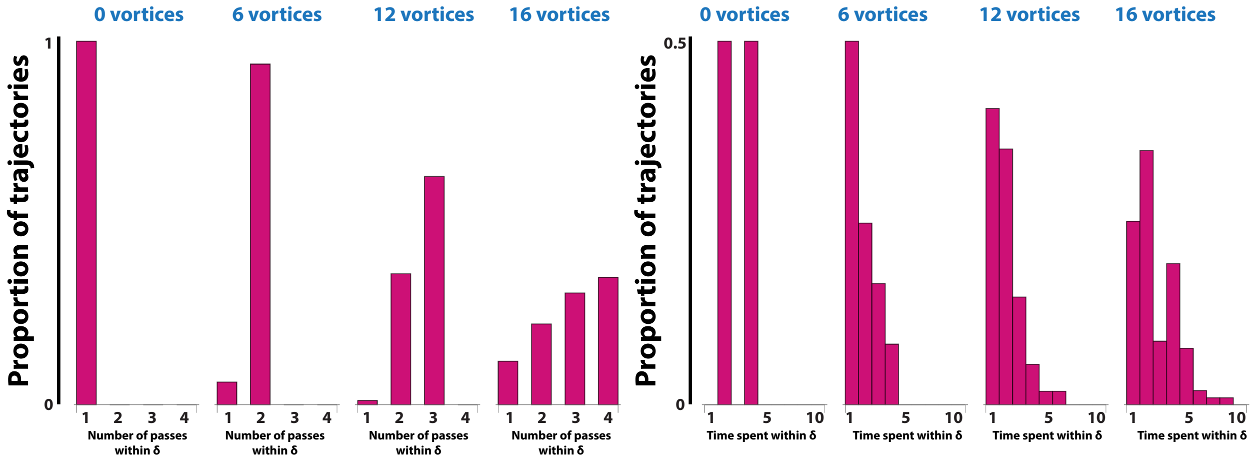


**Figure S8 The effect of vortex number on interception of particles.** Left: Among all particles that pass within $\delta$ of the surface, the number of separate passes near the surface as a function of $n$. Right: For the same simulations, the distribution of total time spent near the surface as a function of $n$. Note that all histograms are normalized to 1, and so for higher numbers of vortices, the additional effect of higher numbers of particles passing within $\delta$ is not visible.

mode" squirmers creates an increase in the capture cross section with $n$. This effect is partly geometric in origin: higher order squirmer models compress parallel incoming trajectories such that a high fraction of incoming particles will pass within the interception distance. However, there are two other effects worth noting:

1. Higher order modes allow particles to take repeated passes near the surface of the swimmer, due to the presence of streamlines that repeatedly approach $-$ defects and then exit along $+$ defects as they pass over the surface.

2. Even in the absence of repeated passes, particles spend a higher fraction of time within the interception distance of the surface. This is due partly to the inverse scaling of $v_{swim}$ with $n$, but at high $n$ additional nonlinear effects emerge.

In order to illustrate the role of these effects, histograms showing the average number of passes near the surface as a function of the number of vortices, as well as the total time spent near the surface, are shown in Figure S8.

### E.1 Comparison with other feeding metrics

For a swimmer passing through a field of particles, the feeding rate is defined as the number of particles encountered per time, $\dot{N}$,

$$\dot{N}(\mathbf{r}, t) = \rho(\mathbf{r}, t)\sigma(t)v_{swim}(t)$$

where $\rho(\mathbf{r}, t)$ is the density of nutrient particles in the fluid, which in general is allowed to vary in both time and space. $\sigma(t)$ represents the swimmer's "isotropic capture cross section," which may vary in time as the swimmer adjusts its capture strategy. For a passive swimmer, $\sigma$ may simply represent the geometric cross section, but for a particle with active boundary conditions it can be larger or smaller. Additionally, the swimmer can modulate its swimming speed, $v_{swim}(t)$. The total amount of food ingested by the swimmer is given by the time integral of $\dot{N}$.

We note that only the nutrient particle density, $\rho$, explicitly depends on space, and so we can compare the instantaneous feeding rate for different instantaneous distributions of nutrients. We first study the case of an initially uniform distribution, which corresponds to the case of either low Peclet number (high nutrient diffusivity or low relative advection speeds) or very high nutrient density (in which case the ciliary capture mechanisms are saturated regardless of spatial gradients in the distribution of food particles).

The instantaneous feeding rate becomes the product of three constants,

$$\dot{N} = \rho\sigma v_{swim}$$

where a volume flux (equivalent to the clearance rate) may be defined as $J = \sigma v_{swim}$. The capture cross-section, $\sigma$, may be analytically calculated for some swimmers, but for the squirmer model it requires numerical techniques as described in Section E.

For this homogenous case, the particle influx per unit time is proportional to $\sigma v_{swim}$,

which is maximized for a first order "treadmill swimmer" for which $\{B_n\} = B_1$ (Figure S9, right panel). Our model and simulations thus agree with the results of Michelin and Lauga,[16] who find that the capture rate of particles per unit time is maximized by swimmers that maximize the first-order swimming mode. This remains true even when Langevin dynamics are added to the trajectories (described below), further confirming Michelin and Lauga's findings that the first-order mode remains optimal even at low Péclet numbers (turquoise trace in the figure). The agreement between the line source simulations and the coupled advection-diffusion system of Michelin and Lauga can be made more explicit by modifying the properties of the interception process. Instead of assigning a fixed capture probability per unit time, the interception can be made infinitely efficient, such that any particle that passes within the interception distance $\delta$ is instantaneously captured. Under these conditions, the general trend in the feeding rate remains the same (yellow and violet traces in the figure)

This suggests that the geometric cross section is less important than the swimming speed for the case of a homogenous environment, $\rho(\mathbf{r}, t) = \rho$, in which the optimal feeding strategy encourages maximal swimming in order to maximize the flux of fresh particles across the swimmer's surface. However, previous experimental work on planktonic larvae has not observed this effect, finding that the larvae of starfish and other echinoderms slow down in order to aggregate near food patches,[17, 18] as do the larvae of krill and copepods,[19–21] and the ciliated veliger larvae of gastropods.[22, 23]

The reason for this discrepancy arises because the unicellular feeders studied by Michelin and Lauga are primarily osmotrophic feeders, which passively absorb nutrients diffusing in their environment—making a discrete version of their feeding efficiency calculation equivalent to finding the first-passage time for an advected Brownian particle to reach the surface of the swimmer. But an established difference between planktonic invertebrate larvae and oceanic bacteria and phytoplankton is that the latter lives in a mostly homogenous nutrient environment (due to diffusion and other processes that rapidly equilibrate spatial gradients), whereas the former have adapted to exploit the "patchiness" of oceanic algae blooms.[24] The

patchiness of oceanic algae distributions at the level of zooplankton is well-established,[25–27] leading one author to even conclude, "For nearly all natural waters, planktonic organisms will be distributed discretely in the fluid mechanical sense. This means that the dynamics of planktonic ecosystems occur among discrete particles, not continuous scalar fields."[28]

Thus while the flux-maximizing feeders studied by Michelin and Lauga may seek maximize their swimming speed, we suggest in the present work that interception feeders may instead optimize their cross-section, leading to a reduced swimming speed in order to collect a greater fraction of total particles intercepted. Intuitively, if food sources are scarce, the optimal feeding strategy should involve maximizing the number of particles gathered during a single pass through a given region of space, necessitating both slower swimming and a larger hydrodynamic cross section.

In addition to numerous studies observing slowing of echinoderm larvae near food patches,[17, 18] direct decreases in the swimming rate of echinoderm larvae in the presence of food particles have been recorded[5, 29] Additionally, comparative studies of related species have led some authors to conclude that a feeding/swimming tradeoff may be observed among distinct echinoderms, and that these features are tied to the geometric extent of the larval body form.[30]

Finally, direct perturbation experiments involving acidification of the growth media in order to create smaller larval cross-sectional area have observed a commensurate decrease in larval feeding rate (but *not* the swimming speed), suggesting that cross-sectional properties must play a role in determining the feeding rate of echinoderm larva.[31, 32]

## F Description of particle capture simulation

For the simulations, a line source of particles was initialized at a fixed distance $5a$ in front of a two-mode swimmer of fixed order $n$, well beyond the point $r_n^s$ described above. The trajectory of each particle as it is advected by the flow of the squirmer was then calculated numerically using the variable-step Adams integrator implemented in Mathematica's NDSolve[] function

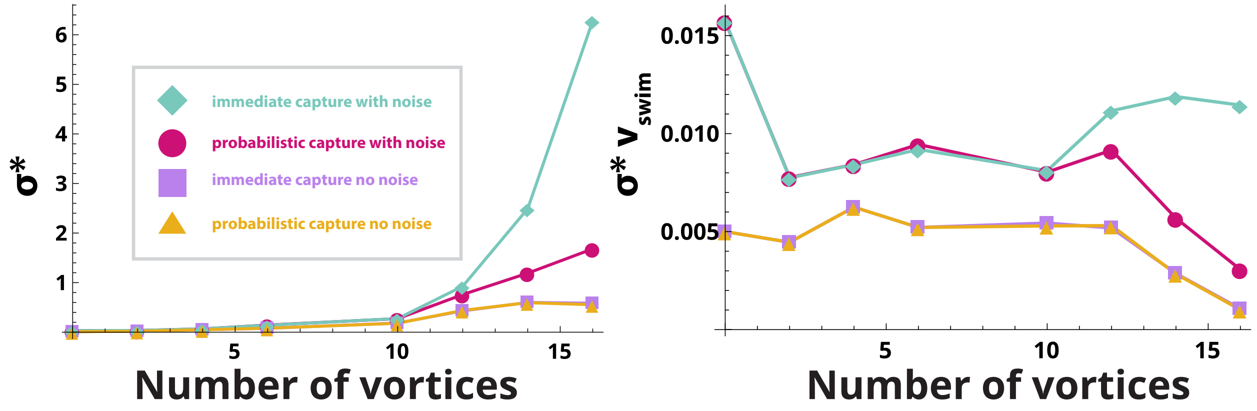


**Figure S9 The distinction between cross section and total particle flux.** The cross section (left) and the feeding rate (right, assuming $\rho = 1$) in a homogenous environment for several variations of the particle capture model tested.

(Figure S10; in the lab frame, these trajectories are the equivalent of the squirmer swimming into a stationary line of particles). Because two-mode squirmers of different $n$ (subject to the two constraints) will swim at different speeds—and thus will have different intrinsic capture abilities due to particles passing over the surface faster or slower—the total simulation time can be rescaled by the swimming speed and body diameter, $t_{sim} = t^*/((1/(2a))B_1)$. $t^*$ is the dimensionless time parameter held fixed for all simulations, and it was chosen to be large enough that most particles eventually cleared the squirmer in all simulations. Rescaling time also reduces systematic errors due to timescale-dependent numerical effects. For each separate simulation, the swimming speed was calculated as $(1/2)B_1$ from (A6) and the capture cross section was calculated using (A9).

### F.1 The effects of random noise

The algae that the larva captures are not perfectly passive tracers; instead, they swim intermittently and may occasionally attempt to change direction—either due to intrinsic stochasticity in their swimming behavior, or due to an escape response. In order to see whether noise in the capture process can affect the positive relationship between the number of vortices and the capture cross section, the advection/capture simulations were repeated

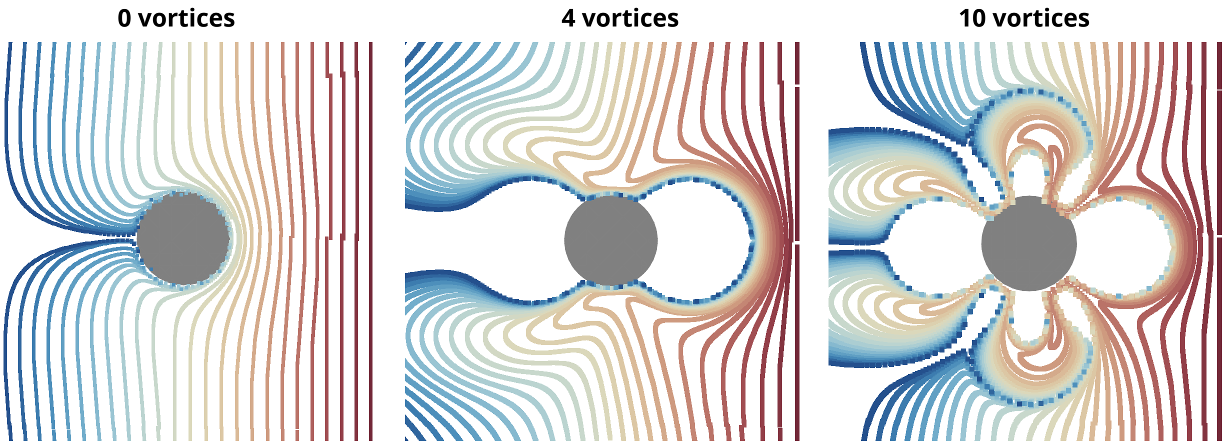


**Figure S10 Advection of passive particles by two-mode swimmers.** The advection of a line of particles by swimmers generating different numbers of vortices. Each color represents a different time, rescaled by the swimming speed to facilitate direct comparison.

with a random noise term added to the squirmer model,

$$\mathbf{u}(x, y, t) = \mathbf{u}^{model}(x(t), y(t)) + k\zeta(t) \tag{A10}$$

where $\mathbf{u}^{model}$ is the original model used in the advection simulation, $k$ is the noise amplitude, and $\zeta$ is a Langevin noise term with the standard properties such as $\langle\zeta(t)\rangle = 0$. Two possible forms of this function were tested:

1. **Brownian noise**. Jumps with amplitudes drawn from a gaussian distribution occur with no preferred timescale. This was chosen based on recent experiments suggesting that over long timescales, swimming phytoplankton undergo diffusion-like run-and-tumble processes[33, 34]

2. **Poisson spike train**. Random "jumps" in velocity in a random direction occur with a well-defined average spacing, $\tau$. This arrival time captures the noticeable intermittency of the algal swimming over short timescales, and is meant to highlight whether differ-

ences in the advection timescale relative to the algae reorientation/response timescale $\tau$ can affect the capture ability. This was chosen based both on observations of the behavior of algae in the advection field, and work suggesting that intermittent algal swimming has extended "runs" as well as intermittent periods of inactivity[35–37]

In the numerical work, each noise source was smoothed for a timescale much smaller than the advection timescale, $a/v_{swim}$, in order to stabilize the numerical simulations. The characteristic timescale for the spike train, $\tau$, was chosen to be an intermediate value so that two-mode swimmers with different speeds encountered significantly different numbers of random events on average.

The results of the simulations with the two different noise sources are shown in Figure S11, and they largely agree with each other. In all cases, the introduction of noise leads to an increase in the capture cross-section that becomes more pronounced with larger numbers of vortices, and this effect scales with the amplitude, $k$, of the noise source. The maximum amplitude tested was determined by the slowest swimming velocity (for the order 8 squirmer with 16 vortices), for which random jumps dominate the system when $k > 2v_{swim}$, leading to nonphysical velocity fluctuations and instability in the numerical integration. Since the algae ($\sim 50$ $\mu$m/s) typically swim slower than the starfish larvae ($\sim 300$ $\mu$m/s), higher noise levels were not considered further.

While the probability of jumping in any direction is equal, jumps into regions with larger expected residence times $\tau$ end up weighing more in the calculation of $\sigma$. Intuitively, this is because some streamlines that pass through the capture region form closed orbits. These are typically inaccessible in simulations without noise, but when noise is introduced particles can jump into closed orbits and repeatedly travel in loops, giving the swimmer many chances to capture them (until they eventually either jump out of the orbit, or they jump to an inner orbit that does not pass within $\delta$ of the surface.

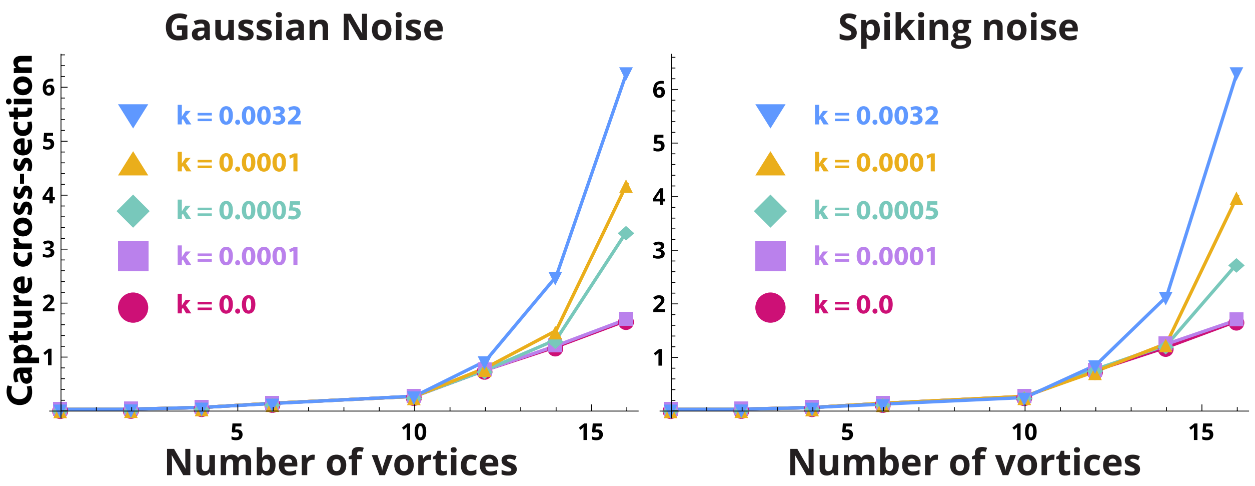


**Figure S11 The effect of random noise on the capture cross section.** Random Brownian noise (left) and "spike" noise with with a fixed average inter-pulse interval (right). The horizontal axis refers to the order of the two-mode squirmer used (parametrized by the number of vortices it generates). The distinct colors/markers refer to different noise amplitudes, $k$ in (A10).

# References


[1] Strathmann, R. R. Culturing larvae of marine invertebrates. *Developmental Biology of the Sea Urchin and Other Marine Invertebrates: Methods and Protocols* 1–25 (2014).

[2] Strathmann, M. F. *Reproduction and development of marine invertebrates of the northern Pacific coast: data and methods for the study of eggs, embryos, and larvae* (University of Washington Press, 1987).

[3] Allison, G. Effects of temporary starvation on larvae of the sea star asterina miniata. *Marine biology* **118**, 255–261 (1994).

[4] Basch, L. & Pearse, J. Consequences of larval feeding environment for settlement and metamorphosis of a temperate echinoderm. *Oceanologica Acta* **19**, 273–285 (1996).

[5] Strathmann, R. R. The feeding behavior of planktotrophic echinoderm larvae: mechanisms, regulation, and rates of suspension feeding. *Journal of Experimental Marine Biology and Ecology* **6**, 109–160 (1971).

[6] Mackie, G., Spencer, A. & Strathmann, R. Electrical activity associated with ciliary reversal in an echinoderm larva. *Nature* (1969).

[7] Hidu, H. & Haskin, H. H. Swimming speeds of oyster larvae crassostrea virginica in different salinities and temperatures. *Estuaries* **1**, 252–255 (1978).

[8] Podolsky, R. & Emlet, R. Separating the effects of temperature and viscosity on swimming and water movement by sand dollar larvae (dendraster excentricus). *Journal of Experimental Biology* **176**, 207–222 (1993).

[9] Taylor, Z. J., Gurka, R., Kopp, G. A. & Liberzon, A. Long-duration time-resolved piv to study unsteady aerodynamics. *IEEE Transactions on Instrumentation and Measurement* **59**, 3262–3269 (2010).

[10] Pedregosa, F. *et al.* Scikit-learn: Machine learning in python. *Journal of Machine Learning Research* **12**, 2825–2830 (2011).

[11] Blake, J. A finite model for ciliated micro-organisms. *Journal of biomechanics* **6**, 133–140 (1973).

[12] Blake, J. Self propulsion due to oscillations on the surface of a cylinder at low Reynolds number. *Bulletin of the Australian Mathematical Society* **5**, 255–264 (1971).

[13] Leal, L. G. *Advanced transport phenomena: fluid mechanics and convective transport processes* (Cambridge University Press, 2007).

[14] Pepper, R. E., Roper, M., Ryu, S., Matsudaira, P. & Stone, H. A. Nearby boundaries create eddies near microscopic filter feeders. *Journal of The Royal Society Interface* rsif20090419 (2009).

[15] Newton, P. K. *The N-vortex problem: analytical techniques*, vol. 145 (Springer Science & Business Media, 2013).

[16] Michelin, S. & Lauga, E. Optimal feeding is optimal swimming for all péclet numbers. *Physics of Fluids (1994-present)* **23**, 101901 (2011).

[17] Metaxas, A. & Young, C. M. Responses of echinoid larvae to food patches of different algal densities. *Marine Biology* **130**, 433–445 (1998).

[18] Sameoto, J. A. & Metaxas, A. Interactive effects of haloclines and food patches on the vertical distribution of 3 species of temperate invertebrate larvae. *Journal of experimental marine biology and ecology* **367**, 131–141 (2008).

[19] Price, H. J. Swimming behavior of krill in response to algal patches: a mesocosm study. *Limnology and Oceanography* **34**, 649–659 (1989).

[20] Tiselius, P. Behavior of acartia tonsa in patchy food environments. *Limnology and Oceanography* **37**, 1640–1651 (1992).

[21] Saiz, E., Tiselius, P., Jonsson, P. R., Verity, P. & Paflenhiifer, G.-A. Experimental records of the effects of food patchiness and predation on egg production of acartia tonsa. *Limnol. Oceanogr* **38**, 280–289 (1993).

[22] Pearce, C. *et al.* Settlement of larvae of the giant scallop, placopecten magellanicus, in 9-m deep mesocosms as a function of temperature stratification, depth, food, and substratum. *Marine biology* **124**, 693–706 (1996).

[23] Gallager, S., Manuel, J., Manning, D. & O'Dor, R. Ontogenetic changes in the vertical distribution of giant scallop larvae, placopecten magellanicus, in 9-m deep mesocosms as a function of light, food, and temperature stratification. *Marine Biology* **124**, 679–692 (1996).

[24] Fenchel, T. Microbial behavior in a heterogeneous world. *Science* **296**, 1068–1071 (2002).

[25] Cassie, R. M. Microdistribution of plankton. *Oceanography and marine biology: an annual review* (1963).

[26] Mitchell, J. G., Yamazaki, H., Seuront, L., Wolk, F. & Li, H. Phytoplankton patch patterns: Seascape anatomy in a turbulent ocean. *Journal of Marine Systems* **69**, 247–253 (2008).

[27] Seymour, J. R., Mitchell, J. G., Pearson, L. & Waters, R. L. Heterogeneity in bacterioplankton abundance from 4.5 millimetre resolution sampling. *Aquatic Microbial Ecology* **22**, 143–153 (2000).

[28] Siegel, D. A. Resource competition in a discrete environment: Why are plankton distributions paradoxical? *Limnology and Oceanography* **43**, 1133–1146 (1998).

[29] Hart, M. W. Particle captures and the method of suspension feeding by echinoderm larvae. *The Biological Bulletin* **180**, 12–27 (1991).

[30] Strathmann, R. R. & Grünbaum, D. Good eaters, poor swimmers: compromises in larval form. *Integrative and Comparative Biology* **46**, 312–322 (2006).

[31] Chan, K. Y. K., Grünbaum, D. & O'Donnell, M. J. Effects of ocean-acidification-induced morphological changes on larval swimming and feeding. *Journal of Experimental Biology* **214**, 3857–3867 (2011).

[32] Chan, K. Y. K., García, E. & Dupont, S. Acidification reduced growth rate but not swimming speed of larval sea urchins. *Scientific reports* **5**, 9764 (2015).

[33] Polin, M., Tuval, I., Drescher, K., Gollub, J. P. & Goldstein, R. E. Chlamydomonas swims with two ?gears? in a eukaryotic version of run-and-tumble locomotion. *Science* **325**, 487–490 (2009).

[34] Locsei, J. T. & Pedley, T. J. Bacterial tracking of motile algae assisted by algal cell's vorticity field. *Microbial ecology* **58**, 63–74 (2009).

[35] Stocker, R. Reverse and flick: Hybrid locomotion in bacteria. *Proceedings of the National Academy of Sciences* **108**, 2635–2636 (2011).

[36] Nurzaman, S. G. *et al.* From levy to brownian: A computational model based on biological fluctuation. *PloS one* **6**, e16168 (2011).

[37] Barbara, G. M. & Mitchell, J. G. Bacterial tracking of motile algae. *FEMS microbiology ecology* **44**, 79–87 (2003).
